# Supplementary material for: $C^3$: Compositional Counterfactual Contrastive Learning for Video-grounded Dialogues
Source: arXiv:2106.08914 source file (2023-08-05)
Supplement: Supplementary file 1 [file additional_result.tex]

\begin{table*}[htbp]
\centering
\small
\begin{tabular}{lcccccc}
\hline
          & d   & h & B-4   & M     & R     & C     \\
          \hline
MTN       & 128 & 8 & 0.376$\pm0.003$ & 0.253$\pm0.001$ & 0.534$\pm0.003$ & 0.996$\pm0.007$ \\
\hline
MTN+$C^3(\mathcal{I}^{+/-})$ & 128 & 8 & 0.398$\pm0.003$ & 0.262$\pm0.001$ & 0.549$\pm0.002$ & 1.040$\pm0.003$ \\
MTN+$C^3(\mathcal{I}^{+/-})$ & 64  & 8 & 0.370$\pm0.002$ & 0.250$\pm0.002$ & 0.530$\pm0.001$ & 0.940$\pm0.004$ \\
MTN+$C^3(\mathcal{I}^{+/-})$ & 128 & 1 & 0.352$\pm0.004$ & 0.242$\pm0.002$ & 0.521$\pm0.002$ & 0.917$\pm0.003$ \\
MTN+$C^3(\mathcal{I}^{+/-})$ & 128 & 2 & 0.389$\pm0.003$ & 0.253$\pm0.001$ & 0.536$\pm0.003$ & 1.018$\pm0.006$ \\
MTN+$C^3(\mathcal{I}^{+/-})$ & 128 & 4 & 0.393$\pm0.002$ & 0.259$\pm0.001$ & 0.545$\pm0.002$ & 1.028$\pm0.007$ \\
\hline
MTN+$C^3(\mathcal{H}^{+/-})$ & 128 & 8 & 0.393$\pm0.003$                     & 0.260$\pm0.003$                     & 0.545$\pm0.001$                     & 1.029 $\pm0.005$                    \\
MTN+$C^3(\mathcal{H}^{+/-})$ & 64  & 8 & 0.372$\pm0.002$                     & 0.248$\pm0.001$                     & 0.527$\pm0.002$                     & 0.937$\pm0.006$                     \\
MTN+$C^3(\mathcal{H}^{+/-})$ & 128 & 1 & 0.351$\pm0.003$                     & 0.232$\pm0.002$                     & 0.503$\pm0.004$                     & 0.882$\pm0.008$                     \\
MTN+$C^3(\mathcal{H}^{+/-})$ & 128 & 2 & 0.386$\pm0.005$                     & 0.251$\pm0.004$                     & 0.534$\pm0.001$                     & 1.000 $\pm0.009$                    \\
MTN+$C^3(\mathcal{H}^{+/-})$ & 128 & 4 & 0.391 $\pm0.002$                    & 0.257$\pm0.001$                     & 0.543$\pm0.001$                     & 1.019$\pm0.005$ \\
\hline
\end{tabular}
\caption{
Additional experiment results with standard deviations on 4 metrics: B-4 (BLEU-4), M (METEOR), R (ROUGE-L), and C(CIDEr). $d$ denotes the embedding dimension and $h$ denotes the number of attention heads.
}
\label{tab:additional_results}
\end{table*}
