# Supplementary material for: $C^3$: Compositional Counterfactual Contrastive Learning for Video-grounded Dialogues
Source: arXiv:2106.08914 source file (2023-08-05)
Supplement: Supplementary file 2 [file dataset_appendix.tex]

\begin{table}[htbp]
%\resizebox{1.0\textwidth}{!} {
\small \centering
\begin{tabular}{lccc}
\hline
\multicolumn{1}{c}{} & \textbf{Train} & \textbf{Val} & \textbf{Test} \\
\hline
\textbf{\#Dialogs}   & 7,659          & 1,787        & 1,710                                \\
\textbf{\#Questions/Answers}     & 153,180        & 35,740       & 13,490                \\
\textbf{\#Words}     & 1,450,754      & 339,006      & 110,252                             \\
\hline
\end{tabular}
%}
\caption{Summary of the AVSD benchmark}
\label{tab:dataset}
%\vspace{-0.1in}
\end{table}
